# Supplementary material for: Relaxation timescales and electron-phonon coupling in optically-pumped YBa$_2$Cu$_3$O$_{6+x}$ revealed by time-resolved Raman scattering
Source: arXiv:2010.15958 ancillary file (2021-12-02)
Supplement: Supplementary file 1 [file apical-supplement.pdf]

# Supplementary Information for "Relaxation timescales and electron-phonon coupling in optically-pumped $YBa_2Cu_3O_{6+x}$ revealed by time-resolved Raman scattering."

## Supplementary Note 1: Time- and energy- resolution of our time-resolved Raman experiment

In order to find time-zero and measure the time-resolution of our experiment we performed a cross-correlation measurement between the 800 nm pump and 400 nm probe. We placed a BBO crystal cut for sum-frequency generation between 400 nm and 800 nm before the sample and measured the intensity of the sum frequency as a function of time delay. Supplementary Figure 1a,b show the results of this

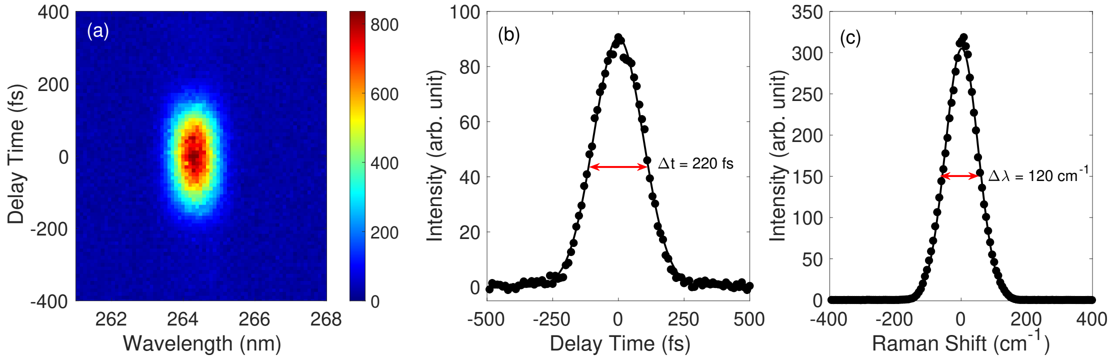


Supplementary Figure 1: Results of a cross-correlation measurement between 800 nm pump and 400 nm probe (a). The resulting time-resolution is 220 fs FWHM (b). The energy resolution, limited by the width in energy of the 400 nm probe, is 120 cm$^{-1}$ (c).

measurement, from which we inferred a time resolution of 220 fs. The main limiting factor in our energy resolution is the spectral width of the 400 nm probe laser. We

fitted the spectrum of the probe laser to a Gaussian peak (Supplementary Figure 1c) and found the resolution to be 120 $\mathrm{cm}^{-1}$ FWHM.

# Supplementary Note 2: Anharmonic decay lifetime dependence on cryostat temperature

FIG. 3 of the main text suggests that 500 fs after the pump pulse arrives, the apical oxygen phonon is no longer hardened and is equilibrated with the electrons. We can then estimate the lifetime for phonon-phonon decay, $\tau$, by fitting the phonon temperature after 500 fs to an exponential function:

$$T_{ph}(t \geq 500 \text{ fs}) = a\mathrm{e}^{-t/\tau} + T_{eq}, \tag{1}$$

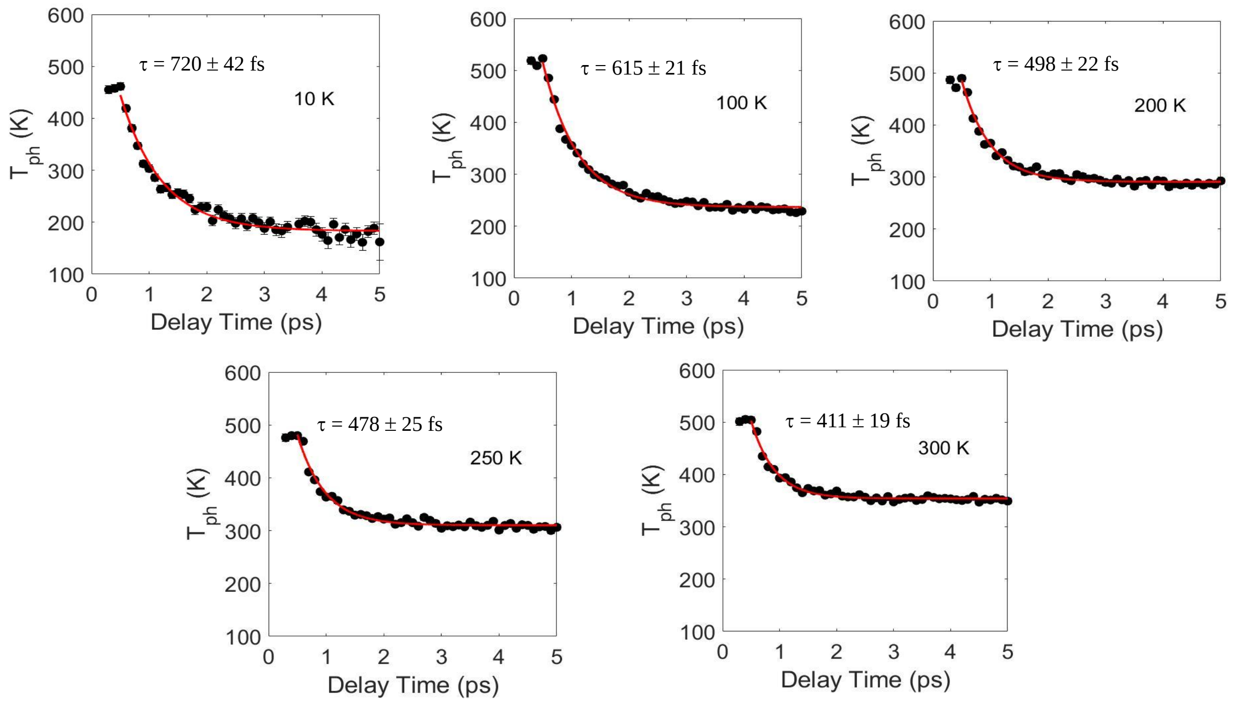


Supplementary Figure 2: Calculated $T_{ph}$ versus delay time for different values of $T_{cryo}$. Red curves are fits of the data at 500 fs and later to a decaying exponential.

The right-hand side of this equation is a constant which is independent of cryostat temperature $T_{cryo}$. The fitted values of $\tau$ are shown in Fig. 1b of the main text as a function of $T_{cryo}$. The variation of $\tau$ with $T_{cryo}$ suggests stronger anharmonic coupling as the cryostat temperature rises.

# Supplementary Note 3: Fits to two-temperature model

We first reproduce here the equations of the two-temperature model used to fit our data:

$$\frac{\partial T_{el}}{\partial t} = -\frac{3\lambda\Omega_0^3}{\hbar\pi k_B^2}\frac{n_{el}-n_h}{T_{el}} + \frac{c_{tot}}{c_{el}(T_{el})}\left(\frac{\Delta T}{2\tau_{pulse}}\mathrm{sech}^2\left(\frac{t}{\tau_{pulse}}\right)\right), \tag{2}$$

$$\frac{\partial T_h}{\partial t} = \frac{c_{el}(T_{el})}{c_h(T_h)}\frac{3\lambda\Omega_0^3}{\hbar\pi k_B^2}\frac{n_{el}-n_h}{T_{el}} - \frac{T_h-T_c}{\tau}, \tag{3}$$

$$\frac{\partial T_c}{\partial t} = \frac{c_h(T_h)}{c_c(T_c)}\frac{T_h-T_c}{\tau}. \tag{4}$$

This model has four parameters: $\Omega_0$, the energy of the phonons; $f$, the fraction of all phonons which are hot; $\lambda$, the strength of the coupling between electrons and hot phonons; and $\tau$, the lifetime for anharmonic phonon decay. Results of fitting our 250 K data with two fixed parameters ($\Omega_0$ and $\tau$) and two free parameters ($f$ and $\lambda$) are presented in Supplementary Figure 3 for many different values of $\Omega_0$ and $\tau$. For values of $\tau \geq 628$ fs, the fits start to decline in quality around delay times of about 0.5 ps. This places a rough upper bound on the lifetime for anharmonic decay. We also note that for fits with $\tau = 328$ fs, the electronic temperature is still significantly higher than the hot phonon temperature at 500 fs. But this contradicts our observation that by 500 fs, the phonon peak energy is back to its equilibrium value. Therefore, the choice of $\tau = 478$ fs is most consistent with our data on the phonon temperature and energy.

For the fits shown in FIG. 3 of the main text, we used the parameters $\Omega_0 = 60$ meV, $\tau = 478$ fs, $f = 0.137$, and $\lambda = 0.065$ which correspond to the fit in the seventh panel of Supplementary Figure 3.

The similar fitting of Supplementary Figure 3 is also carried out for other cryostat temperatures. In Supplementary Figure 4, the fit results of temperature data are shown with two free parameters ($f$ and $\lambda$) only for $\Omega_0$=60 meV. These values of $\tau$ and $\lambda$ are used in the main text in FIG. 1b.

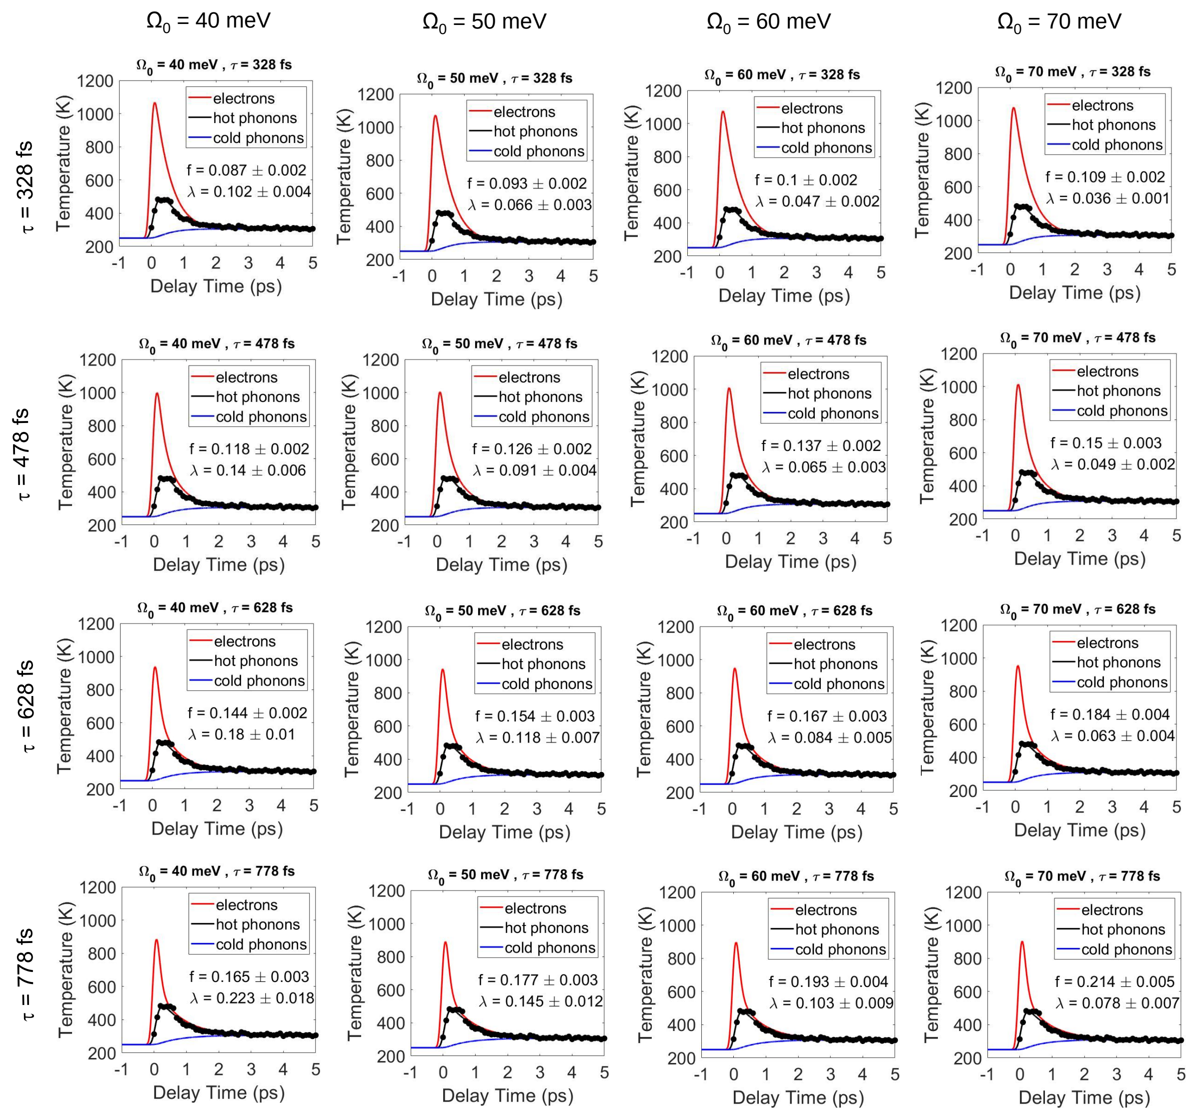


Supplementary Figure 3: Fitting results of 250 K data with two free parameters ($f$ and $\lambda$). While $f$ and $\lambda$ were free, we chose fixed values of $\Omega_0$ and $\tau$ for each fit. In general, it seems that changing $\Omega_0$ doesn't affect the quality of the fit. Values of $\tau \geq 628$ fs result in poorer fits to the data around 0.5 ps. Values of $\tau \ll 478$ fs lead to the electrons and hot phonons equilibrating at times later than what is suggested by our data on the phonon energy in FIG. 3b of the main text.

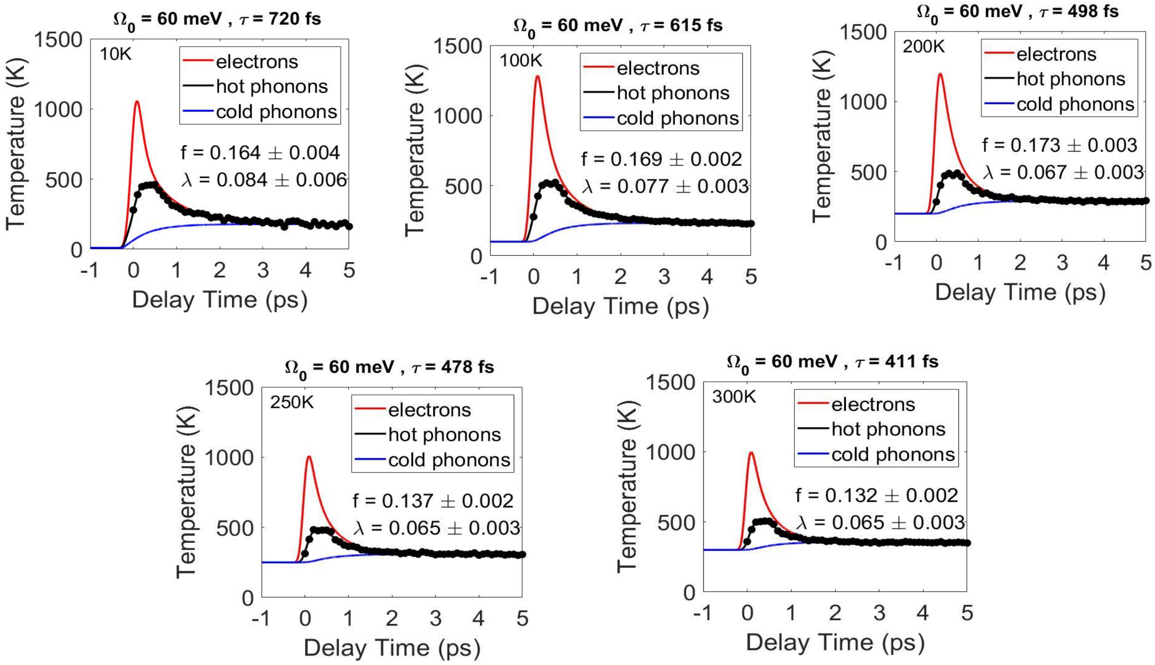


Supplementary Figure 4: Results of two temperature model fit of the data corresponding to all the cryostat temperatures with two free parameters ($f$ and $\lambda$) for $\Omega_0$=60 meV .
